# Supplementary material for: Multimodal End-to-End Autonomous Driving
Source: arXiv:1906.03199 source file (2020-10-25)
Supplement: Supplementary file 1 [file appendix.tex]

% if have a single appendix:
\thispagestyle{empty}
\appendix[Network Architectures]

% or
%\appendix  % for no appendix heading
% do not use \section anymore after \appendix, only \section*
% is possibly needed

% use appendices with more than one appendix
% then use \section to start each appendix
% you must declare a \section before using any
% \subsection or using \label (\appendices by itself
% starts a section numbered zero.)
%

%\appendices
%\section{Proof of the First Equation}

In this Appendix, we provide details on the CIL architecures used in this work. In all the tables we use the same terminology. M is the number of input perception channels. M=3 for RGB, M=1 for depth (D) only, M=4 for RGBD. As measurement input, only the current speed of the vehicle is used. The output are the steering angle, the throttle and the braking forces. There are four action branches. The speed branch is only used at training time for performing multi-task learning with the action branches. ReLU nonlinearities are applied after all hidden layers, and batch normalization is performed after convolutional layers. No dropout is applied after convolutional layers. Tables \ref{tab:configuration}, \ref{tab:MidFusionConfiguration}, and \ref{tab:LateFusionConfiguration}, summarize the details for early, mid and late fusion CIL architectures.

\begin{table}[h!]
\begin{center}
\caption{CIL network details (original and early fusion).}
\label{tab:configuration}
\resizebox{\columnwidth}{!}{
\begin{scriptsize}
\begin{tabular}{cccccc}
\toprule
       & Input     & Output   & Num. of &        &        \\
Module & Dimension & Channels & Kernels & Stride & Dropout\\
\noalign{\smallskip}
\midrule
        & 200 $\times$ 88 $\times$ M & 32 & 5 & 2 & 0.0\\
        & 98 $\times$ 48 $\times$ 32 & 32 & 3 & 1 & 0.0\\
        & 96 $\times$ 46 $\times$ 32 & 64 & 3 & 2 & 0.0\\
        & 47 $\times$ 22 $\times$ 64 & 64 & 3 & 1 & 0.0\\
 Perception & 45 $\times$ 20 $\times$ 64 & 128 & 3 & 2 & 0.0\\
        & 22 $\times$ 9 $\times$ 128 & 128& 3 & 1 & 0.0\\
        & 20 $\times$ 7 $\times$ 128 & 256 & 3 & 2 & 0.0\\
        & 9 $\times$ 3 $\times$ 256 & 256 & 3 & 1 & 0.0\\
        & 7 $\times$ 1 $\times$ 256 & 512 & - & - & 0.0\\ 
        & 512 & 512 & - & - & 0.0 \\
\midrule
  Measurement  & 1 & 128 & - & -  & 0.0 \\
        & 128 & 128 & - & - & 0.0 \\
\midrule
 Join & 512+128  & 512 & - & - & 0.3 \\
\midrule
              & 512  & 256 & - & - & 0.5\\
Action Branch & 256  & 256 & - & -  & 0.5\\
              & 256  & 3 & - & - & 0.0\\
\midrule
        & 512  & 256 & - & - & 0.5\\
 Speed Branch & 256  & 256 & - & -  & 0.5\\
        & 256  & 1 & - & -  & 0.0\\ 
\bottomrule
\end{tabular}
\end{scriptsize}
}
\end{center}
\end{table}

\begin{table}[t!]
\begin{center}
\caption{Mid Fusion Network Details}
\label{tab:MidFusionConfiguration}
\resizebox{\columnwidth}{!}{
\begin{scriptsize}
\begin{tabular}{cccccc}
\toprule
       & Input     & Output   & Num. of &        &        \\
Module & Dimension & Channels & Kernels & Stride & Dropout\\
\noalign{\smallskip}
\midrule
        & 200 $\times$ 88 $\times$ 3 & 32 & 5 & 2 & 0.0\\
        & 98 $\times$ 48 $\times$ 32 & 32 & 3 & 1 & 0.0\\
        & 96 $\times$ 46 $\times$ 32 & 64 & 3 & 2 & 0.0\\
        & 47 $\times$ 22 $\times$ 64 & 64 & 3 & 1 & 0.0\\
 Perception (RGB) & 45 $\times$ 20 $\times$ 64 & 128 & 3 & 2 & 0.0\\
        & 22 $\times$ 9 $\times$ 128 & 128& 3 & 1 & 0.0\\
        & 20 $\times$ 7 $\times$ 128 & 256 & 3 & 2 & 0.0\\
        & 9 $\times$ 3 $\times$ 256 & 256 & 3 & 1 & 0.0\\
        & 7 $\times$ 1 $\times$ 256 & 512 & - & - & 0.0\\ 
        & 512 & 512 & - & - & 0.0 \\
\midrule
        & 200 $\times$ 88 $\times$ 1 & 32 & 5 & 2 & 0.0\\
        & 98 $\times$ 48 $\times$ 32 & 32 & 3 & 1 & 0.0\\
        & 96 $\times$ 46 $\times$ 32 & 64 & 3 & 2 & 0.0\\
        & 47 $\times$ 22 $\times$ 64 & 64 & 3 & 1 & 0.0\\
 Perception (Depth) & 45 $\times$ 20 $\times$ 64 & 128 & 3 & 2 & 0.0\\
        & 22 $\times$ 9 $\times$ 128 & 128& 3 & 1 & 0.0\\
        & 20 $\times$ 7 $\times$ 128 & 256 & 3 & 2 & 0.0\\
        & 9 $\times$ 3 $\times$ 256 & 256 & 3 & 1 & 0.0\\
        & 7 $\times$ 1 $\times$ 256 & 512 & - & - & 0.0\\ 
        & 512 & 512 & - & - & 0.0 \\
\midrule
  Measurement  & 1 & 128 & - & -  & 0.0 \\
        & 128 & 128 & - & - & 0.0 \\
\midrule
 Join & 512+512+128  & 512 & - & - & 0.3 \\
\midrule
              & 512  & 256 & - & - & 0.5\\
Action Branch & 256  & 256 & - & -  & 0.5\\
              & 256  & 3 & - & - & 0.0\\
\midrule
        & 512  & 256 & - & - & 0.5\\
 Speed Branch & 256  & 256 & - & -  & 0.5\\
        & 256  & 1 & - & -  & 0.0\\ 
\bottomrule
\end{tabular}
\end{scriptsize}
}
\end{center}
\end{table}

\begin{table}
\begin{center}
\caption{Late Fusion Network Details}
\label{tab:LateFusionConfiguration}
\resizebox{\columnwidth}{!}{
\begin{scriptsize}
\begin{tabular}{cccccc}
\toprule
       & Input     & Output   & Num. of &        &        \\
Module & Dimension & Channels & Kernels & Stride & Dropout\\
\noalign{\smallskip}
\midrule
        & 200 $\times$ 88 $\times$ 3 & 32 & 5 & 2 & 0.0\\
        & 98 $\times$ 48 $\times$ 32 & 32 & 3 & 1 & 0.0\\
        & 96 $\times$ 46 $\times$ 32 & 64 & 3 & 2 & 0.0\\
        & 47 $\times$ 22 $\times$ 64 & 64 & 3 & 1 & 0.0\\
 Perception (RGB) & 45 $\times$ 20 $\times$ 64 & 128 & 3 & 2 & 0.0\\
        & 22 $\times$ 9 $\times$ 128 & 128& 3 & 1 & 0.0\\
        & 20 $\times$ 7 $\times$ 128 & 256 & 3 & 2 & 0.0\\
        & 9 $\times$ 3 $\times$ 256 & 256 & 3 & 1 & 0.0\\
        & 7 $\times$ 1 $\times$ 256 & 512 & - & - & 0.0\\ 
        & 512 & 512 & - & - & 0.0 \\
\midrule
        & 200 $\times$ 88 $\times$ 1 & 32 & 5 & 2 & 0.0\\
        & 98 $\times$ 48 $\times$ 32 & 32 & 3 & 1 & 0.0\\
        & 96 $\times$ 46 $\times$ 32 & 64 & 3 & 2 & 0.0\\
        & 47 $\times$ 22 $\times$ 64 & 64 & 3 & 1 & 0.0\\
 Perception (Depth) & 45 $\times$ 20 $\times$ 64 & 128 & 3 & 2 & 0.0\\
        & 22 $\times$ 9 $\times$ 128 & 128& 3 & 1 & 0.0\\
        & 20 $\times$ 7 $\times$ 128 & 256 & 3 & 2 & 0.0\\
        & 9 $\times$ 3 $\times$ 256 & 256 & 3 & 1 & 0.0\\
        & 7 $\times$ 1 $\times$ 256 & 512 & - & - & 0.0\\ 
        & 512 & 512 & - & - & 0.0 \\
\midrule
Measurement (RGB)  & 1 & 128 & - & -  & 0.0 \\
        & 128 & 128 & - & - & 0.0 \\
\midrule
Measurement (Depth)  & 1 & 128 & - & -  & 0.0 \\
        & 128 & 128 & - & - & 0.0 \\
\midrule
 Join (RGB) & 512+128  & 512 & - & - & 0.3 \\
\midrule
 Join (Depth) & 512+128  & 512 & - & - & 0.3 \\
\midrule
              & 512  & 256 & - & - & 0.5\\
Action Branch (RGB) & 256  & 256 & - & -  & 0.5\\
              & 256  & 3 & - & - & 0.0\\
\midrule
              & 512  & 256 & - & - & 0.5\\
Action Branch (Depth) & 256  & 256 & - & -  & 0.5\\
              & 256  & 3 & - & - & 0.0\\
\midrule
 Join (Streams)&  3+3 & 256 & - & - & 0.0 \\
\midrule
    & 256 & 128 & - & - & 0.0 \\
Final Action & 128 & 128 & - & - & 0.0 \\
    & 128 & 3 & - & - & 0.0 \\
\midrule
        & 512  & 256 & - & - & 0.5 \\
 Speed Branch (RGB) & 256  & 256 & - & -  & 0.5 \\
        & 256  & 1 & - & -  & 0.0 \\ 
\midrule
       & 512  & 256 & - & - & 0.5 \\
 Speed Branch (Depth) & 256  & 256 & - & -  & 0.5\\
        & 256  & 1 & - & -  & 0.0 \\ 
\midrule
 Join (Speeds) &  1+1 & 256 & - & - & 0.0 \\
\midrule
    & 256 & 128 & - & - & 0.0 \\
Final Speed & 128 & 128 & - & - & 0.0 \\
    & 128 & 1 & - & - & 0.0 \\
\bottomrule
\end{tabular}
\end{scriptsize}
}
\end{center}
\end{table}
